# Supplementary material for: Neural Networks Enhancement with Logical Knowledge
Source: arXiv:2009.06087 source file (2021-10-18)
Supplement: Supplementary file 1 [file appendix1.tex]

\chapter{Details of experiments}
\label{app:details}

Totally optional
\section{Setup of Experiment 1}
\section{Detailed results}
